# Supplementary material for: Bayesian inference for treatment effects under nested subsets of controls
Source: arXiv:2001.07256 source file (2022-09-02)
Supplement: Supplementary file 1 [file analytical-results.tex]

\section{Identifying assumptions}
\label{sec:ident-assumpt}

\n{Rewrite for generic Z}

To nonparametrically identify the causal effect of $Z$, the set of controls $X$ must be sufficient such that
\begin{align}\label{eq:ignorability} Y_i(z) \ind Z_i \mid X_i = x_i
\end{align}
where $Y(z')$ denotes the outcome when the treatment is assigned to $Z=z'$.  This is the weak unconfoundedness assumption of \cite{hirano2004propensity}, and is closely related to the exogeneity assumption more commonly found in the econometric literature which is expressed as:
\begin{align*} \cov(Z_i, \epsilon_i \mid X_i) = 0.
\end{align*}
in the context of a regression model with errors $\epsilon_i$.
Further, the assumption of overlap or positivity must hold, that is
\begin{align*} \pi(z \mid x) > 0 \,\,\;\; \forall \,\, z, x
\end{align*}
where $\pi(z \mid x)$ is the conditional density of $z$ given $x$.  Recent work has shown that weaker forms of this assumption can still allow for identification of causal estimands like incremental treatment effects
%\begin{align*}
%\E(Y(Z + \Delta Z) - Y(Z) \mid X) = \tau \cdot \Delta Z.
%\end{align*} 
defined above \citep{wu,binyu}.  Throughout the paper we assume that the incremental causal effects in Eq~\eqref{eq:delta} are nonparametrically identified under these assumptions, and in particular that we measured all the confounding variables.\sw{}

\section{Deriving analytical results for projected posterior with a
  flat prior}
\label{sec:analyt-results-from}

Consider the matrix $\Xt$ of reduced columns of $X = [\Xt \quad \Xd]$
(i.e., remove the $\Xd$ columns of $X$) with corresponding vector
$\betat$, and corresponding concatenations $\Wt = [Z \quad \Xt]$ and
$\psit = [\tau \quad\betat]$.  Denote the projection matrix for $W$
to be $P_W:=W(W^\trans W)^{-1}W^\trans$.  Note that $\Wt$ is in the
column space of $W$, so $P\Wt = \Wt$.

\subsection{Main matrix inverse decomposition}

Block matrix inverse identity:
\begin{align}
  \begin{bmatrix}
    \mathbf{A} & \mathbf{B} \\
    \mathbf{C} & \mathbf{D}
  \end{bmatrix}^{-1} &= \begin{bmatrix}
     \mathbf{A}^{-1} + \mathbf{A}^{-1}\mathbf{B}(\mathbf{D} - \mathbf{CA}^{-1}\mathbf{B})^{-1}\mathbf{CA}^{-1} &
      -\mathbf{A}^{-1}\mathbf{B}(\mathbf{D} - \mathbf{CA}^{-1}\mathbf{B})^{-1} \nonumber \\
    -(\mathbf{D}-\mathbf{CA}^{-1}\mathbf{B})^{-1}\mathbf{CA}^{-1} &
       (\mathbf{D} - \mathbf{CA}^{-1}\mathbf{B})^{-1}
     \end{bmatrix} \\
  &= \begin{bmatrix}
     (\mathbf{A} - \mathbf{BD}^{-1}\mathbf{C})^{-1} &
      -(\mathbf{A}-\mathbf{BD}^{-1}\mathbf{C})^{-1}\mathbf{BD}^{-1} \\
    -\mathbf{D}^{-1}\mathbf{C}(\mathbf{A} - \mathbf{BD}^{-1}\mathbf{C})^{-1} &
       \quad \mathbf{D}^{-1} + \mathbf{D}^{-1}\mathbf{C}(\mathbf{A} - \mathbf{BD}^{-1}\mathbf{C})^{-1}\mathbf{BD}^{-1}
  \end{bmatrix} \label{eq:matrix-ident}
\end{align}

Find the inverse for the covariance matrix using
Eq.~\eqref{eq:matrix-ident}: 
\begin{align}
  (W^\trans W)^{-1} &= 
                      \left(
                      \begin{bmatrix}
                        \Wt^\trans \\
                        \Xd^\trans
                      \end{bmatrix}
  \begin{bmatrix}
    \Wt & \Xd
  \end{bmatrix}
          \right)^{-1} \nonumber \\
  &= 
    \begin{bmatrix}
      \Wt^\trans \Wt & \Wt^\trans \Xd \\
      \Xd^\trans \Wt & \Xd^\trans \Xd
    \end{bmatrix}^{-1} \nonumber \\
                    &=: Q \nonumber \\
                    &=
                      \begin{bmatrix}
                        Q_{11} & Q_{12} \\
                        Q_{21} & Q_{22}
                      \end{bmatrix} \label{eq:Q-decomp}
\end{align}

With
\begin{align*}
  Q_{11} &= (\Wt^\trans \Wt - \Wt^\trans \Xd (\Xd^\trans \Xd)^{-1} \Xd^\trans\Wt )^{-1} \\
  Q_{12} &= -(\Wt^\trans \Wt - \Wt^\trans \Xd (\Xd^\trans \Xd)^{-1} \Xd^\trans\Wt )^{-1} \Wt^\trans \Xd (\Xd^\trans \Xd)^{-1} \\
  Q_{21} &= - (\Xd^\trans \Xd)^{-1} \Wt^\trans \Xd (\Wt^\trans \Wt - \Wt^\trans \Xd (\Xd^\trans \Xd)^{-1} \Xd^\trans\Wt )^{-1} \\
  Q_{22} &= (\Xd^\trans \Xd)^{-1} + (\Xd^\trans \Xd)^{-1} \Wt^\trans \Xd (\Wt^\trans \Wt - \Wt^\trans \Xd (\Xd^\trans \Xd)^{-1} \Xd^\trans\Wt )^{-1} \Wt^\trans \Xd (\Xd^\trans \Xd)^{-1}
\end{align*}

Note that $Q_{11}$ is the component corresponding to the $\Wt$ components, and reduces to
\begin{align}
  Q_{11} &= (\Wt^\trans \Wt - \Wt^\trans \Xd (\Xd^\trans \Xd)^{-1} \Xd^\trans\Wt )^{-1} \nonumber \\
         &= [\Wt^\trans (\I - \Xd \{ \Xd^\trans \Xd \}^{-1}\Xd) \Wt]^{-1} \nonumber \\
         &= [\Wt^\trans (\I - P_{\Xd}) \Wt]^{-1} \label{eq:Q11}
\end{align}

Where $P_{\Xd} = \Xd (\Xd^\trans \Xd)^{-1} \Xd^\trans$ is the
projection matrix for $\Xd$. And the other blocks reduce to
\begin{align}
  Q_{12} &= -(\Wt^\trans \Wt - \Wt^\trans \Xd (\Xd^\trans \Xd)^{-1} \Xd^\trans\Wt )^{-1} \Wt^\trans \Xd (\Xd^\trans \Xd)^{-1} \nonumber \\
         &= -[\Wt^\trans (\I - P_{\Xd}) \Wt]^{-1} \Wt^\trans \Xd (\Xd^\trans \Xd)^{-1} \label{eq:Q12} \\
         &= - Q_{11} \Wt^\trans \Xd (\Xd^\trans \Xd)^{-1} \label{eq:Q12-Q11}
\end{align}
\begin{align*}
  Q_{21} &= - (\Xd^\trans \Xd)^{-1} \Wt^\trans \Xd (\Wt^\trans \Wt - \Wt^\trans \Xd (\Xd^\trans \Xd)^{-1} \Xd^\trans\Wt )^{-1} \\
  &= - (\Xd^\trans \Xd)^{-1} \Wt^\trans \Xd [\Wt^\trans (\I - P_{\Xd}) \Wt]^{-1}
\end{align*}
\begin{align*}
  Q_{22} &= (\Xd^\trans \Xd)^{-1} + (\Xd^\trans \Xd)^{-1} \Wt^\trans \Xd (\Wt^\trans \Wt - \Wt^\trans \Xd (\Xd^\trans \Xd)^{-1} \Xd^\trans\Wt )^{-1} \Wt^\trans \Xd (\Xd^\trans \Xd)^{-1} \\
  &= (\Xd^\trans \Xd)^{-1} + (\Xd^\trans \Xd)^{-1} \Wt^\trans \Xd [\Wt^\trans (\I - P_{\Xd}) \Wt]^{-1} \Wt^\trans \Xd (\Xd^\trans \Xd)^{-1}
\end{align*}

%Full matrix in \texttt{tiny} text: \tiny
%\begin{align*}
%      \begin{bmatrix}
%      (\Wt^\trans \Wt - \Wt^\trans \Xd (\Xd^\trans \Xd)^{-1} \Xd^\trans\Wt )^{-1} &
%      -(\Wt^\trans \Wt - \Wt^\trans \Xd (\Xd^\trans \Xd)^{-1} \Xd^\trans\Wt )^{-1} \Wt^\trans \Xd (\Xd^\trans \Xd)^{-1} \\
%      - (\Xd^\trans \Xd)^{-1} \Wt^\trans \Xd (\Wt^\trans \Wt - \Wt^\trans \Xd (\Xd^\trans \Xd)^{-1} \Xd^\trans\Wt )^{-1} &
%      (\Xd^\trans \Xd)^{-1} + (\Xd^\trans \Xd)^{-1} \Wt^\trans \Xd (\Wt^\trans \Wt - \Wt^\trans \Xd (\Xd^\trans \Xd)^{-1} \Xd^\trans\Wt )^{-1} \Wt^\trans \Xd (\Xd^\trans \Xd)^{-1}
%    \end{bmatrix}
%\end{align*}

\normalsize

\subsection{Comparing mean vectors}

\paragraph{Marginal from full model}

The posterior mean from the full model is as follows, and then using
Eqs.~\eqref{eq:Q-decomp}, \eqref{eq:Q11}, \eqref{eq:Q12}, and
\eqref{eq:Q12-Q11} gives
\begin{align*}
  \hat \psi
  &= (W^\trans W)^{-1} W^\trans Y \\
  &=
    \begin{bmatrix}
      Q_{11} & Q_{12} \\
      Q_{21} & Q_{22}
    \end{bmatrix} W^\trans Y \\
  &=
    \begin{bmatrix}
      Q_{11} & Q_{12} \\
      Q_{21} & Q_{22}
    \end{bmatrix}
               \begin{bmatrix}
                 \Wt^\trans \\
                 \Xd^\trans
               \end{bmatrix} Y
\end{align*}

The marginal mean vector for the components corresponding to $\Wt$ is
\begin{align*}
  \hat \psi_{\Wt}
  &= (Q_{11} \Wt^\trans + Q_{12} \Xd^\trans)Y \\
  &= (Q_{11} \Wt^\trans + Q_{11}[-\Wt^\trans \Xd (\Xd^\trans \Xd)^{-1}]\Xd^\trans) Y \\
  &= Q_{11} \Wt^\trans (\I - P_{\Xd}) Y \\
  &= [\Wt^\trans (\I - P_{\Xd}) \Wt]^{-1} \Wt^\trans (\I - P_{\Xd}) Y
\end{align*}

If $\Wt$ is orthogonal to $\Xd$, then $P_{\Xd} \Wt = 0$, and
\begin{align*}
  [\Wt^\trans (\I - P_{\Xd}) \Wt]^{-1} \Wt^\trans (\I - P_{\Xd}) Y
  &= (\Wt^\trans \Wt)^{-1} \Wt^\trans Y
\end{align*}

\paragraph{Projection}

Let $P_W = {W (W^\trans W)^{-1} W^\trans}$ be the projection matrix of
$W$.

Perform the projection
\begin{align*}
  \psit &= {(\Wt^\trans \Wt)^{-1} \Wt^\trans W} \psi
\end{align*}

Because $\Wt$ is in the column space of $W$, the projected posterior
mean is
\begin{align*}
  \text{E}(\psit \mid Y) &= (\Wt^\trans \Wt)^{-1} \Wt^\trans
                           {W (W^\trans W)^{-1} W^\trans} Y \\
                         &= (\Wt^\trans \Wt)^{-1} \Wt^\trans
                           P_W Y \\
                         &= (\Wt^\trans \Wt)^{-1} \Wt^\trans Y
\end{align*}

\paragraph{Refit}

\begin{align*}
  \hat{\psit} &= (\Wt^\trans \Wt)^{-1} \Wt^\trans Y
\end{align*}

\subsection{Comparing covariance matrices}

\paragraph{Marginal from full model}

\begin{align*}
  \cov(\psi \mid Y) &= \sigma_\epsilon^2 (W^\trans W)^{-1}
\end{align*}
So the marginal covariance matrix for the components of $\Wt$, using
Eq.~\eqref{eq:Q-decomp} and Eq.~\eqref{eq:Q11}, is
\begin{align*}
  \cov_\text{marg}(\psit \mid Y)
  &= \sigma^2_\epsilon [\Wt^\trans (\I - P_{\Xd}) \Wt]^{-1}
\end{align*}

Note that using the Woodbury matrix identity,
\begin{align*}
  & [\Wt^\trans (\I - P_{\Xd}) \Wt]^{-1} \\
  = &[\Wt^\trans \Wt - \Wt^\trans P_{\Xd} \Wt]^{-1} \\
  = & [\Wt^\trans \Wt]^{-1} -
  [\Wt^\trans \Wt]^{-1} \Wt^\trans
  (P_{\Xd}^{-1} + \Wt [\Wt^\trans \Wt]^{-1} \Wt^\trans)^{-1}
      \Wt [\Wt^\trans \Wt]^{-1} \\
  = & [\Wt^\trans \Wt]^{-1} -
  [\Wt^\trans \Wt]^{-1} \Wt^\trans
  (P_{\Xd}^{-1} + P_{\Wt})^{-1}
  \Wt [\Wt^\trans \Wt]^{-1}
\end{align*}

If $\Wt$ is orthogonal to $\Xd$, then $P_{\Xd} \Wt = 0$, and
\begin{align*}
  \sigma^2_\epsilon [\Wt^\trans (\I - P_{\Xd}) \Wt]^{-1}
  &= \sigma^2_\epsilon [\Wt^\trans \Wt]^{-1}
\end{align*}

\paragraph{Projection}

From Eq.~\eqref{eq:proj-cov},
\begin{align*}
  \cov_\text{proj}(\psit \mid Y) &= \sigma_\epsilon^2 (\Wt^\trans \Wt)^{-1}
\end{align*}

\paragraph{Refit}

\begin{align*}
  \cov_\text{refit}(\psit \mid Y) &= \sigma^2_{\text{refit}} (\Wt^\trans \Wt)^{-1}
\end{align*}

\subsubsection{Considering only $\tau$}

$P_Z = Z(Z^\trans Z)^{-1}Z^\trans = ZZ^\trans / SSZ$, $SSZ = \sum_i Z_i^2$

\paragraph{Marginal}

\begin{align*}
  \cov_\text{marg}(\tau \mid Y)
  &= \sigma^2_\epsilon [Z^\trans (\I - P_{X}) Z]^{-1} \\
  &= \sigma^2_\epsilon \left\{
     [Z^\trans Z]^{-1} -
  [Z^\trans Z]^{-1} Z^\trans
  (P_{X}^{-1} + P_{Z})^{-1}
  Z [Z^\trans Z]^{-1}
    \right\}
\end{align*}

Using the Sherman-Morrison formula, 
\begin{align*}
  (P_{X}^{-1} + P_{Z})^{-1} &= P_X - \frac{\frac{1}{SSZ} P_X Z Z^\trans P_X}{1 + \frac{1}{SSZ} Z^\trans P_X Z}
\end{align*}

\paragraph{Projection}

\begin{align*}
  \cov_\text{proj}(\tau \mid Y)
  &= \sigma^2_\epsilon [Z^\trans(\I - P_{\Xt}) Z]^{-1} \\
  &= \sigma^2_\epsilon \left\{
     [Z^\trans Z]^{-1} -
  [Z^\trans Z]^{-1} Z^\trans
  (P_{\Xt}^{-1} + P_{Z})^{-1}
  Z [Z^\trans Z]^{-1}
    \right\}
\end{align*}

\paragraph{The difference, ignoring factor of $\sigma^2_\epsilon$}

\begin{align*}
  &\cov_\text{marg}(\tau \mid Y) - \cov_\text{proj}(\tau \mid Y) \\
  % =&\sigma^2_\epsilon
  %   \left\{
  %   [Z^\trans Z]^{-2} Z^\trans [(P_{\Xt}^{-1} + P_{Z})^{-1} - (P_{X}^{-1} + P_{Z})^{-1}] Z
  %   \right\} \\
  % =&\sigma^2_\epsilon
  %   \left\{
  %   [Z^\trans Z]^{-2} Z^\trans 
  %   \left[
  %   \left(
  %   P_{\Xt} - \frac{\frac{1}{SSZ} P_{\Xt} Z Z^\trans P_{\Xt}}{1 + \frac{1}{SSZ} Z^\trans P_{\Xt} Z}
  %   \right) -
  %   \left(
  %   P_X - \frac{\frac{1}{SSZ} P_X Z Z^\trans P_X}{1 + \frac{1}{SSZ} Z^\trans P_X Z}
  %   \right)
  %   \right] Z
  % \right\}
       =& \frac{1}{Z^\trans (\I - P_X)Z} - \frac{1}{Z^\trans (\I - P_{\Xt})Z} \\
  =& \frac{{Z^\trans (\I - P_{\Xt})Z} - {Z^\trans (\I - P_X)Z}}
     {{Z^\trans (\I - P_X)Z} \cdot {Z^\trans (\I - P_{\Xt})Z}} \\
  =& \frac{Z^\trans[(\I - P_{\Xt}) - (\I - P_X)]Z}
     {{Z^\trans (\I - P_X)Z} \cdot {Z^\trans (\I - P_{\Xt})Z}} \\
  =& \frac{Z^\trans (P_{X} - P_{\Xt}) Z}
     {{Z^\trans (\I - P_X)Z} \cdot {Z^\trans (\I - P_{\Xt})Z}} \\
\end{align*}

Note the idempotency $P_X = P_X P_X$, and $P_X = P_X P_{\Xt} P_X$ because
$\Xt$ is in the column space of $X$, so then the numerator is
\begin{align*}
  Z^\trans (P_{X} - P_{\Xt}) Z
  &= Z^\trans (P_{X} P_{X} - P_X P_{\Xt} P_X) Z \\
  &= Z^\trans P_X (\I - P_{\Xt}) P_X Z > 0
\end{align*}
when $P_X Z \neq 0$, because $\I - P_{\Xt}$ is positive definite.

%%% Local Variables:
%%% mode: latex
%%% TeX-master: "../main"
%%% End:
