# Supplementary material for: Bayesian inference for treatment effects under nested subsets of controls
Source: arXiv:2001.07256 source file (2022-09-02)
Supplement: Supplementary file 2 [file joint-mv-gaussian.tex]

\section{Joint multivariate Gaussian results}

\paragraph{Joint of $z$ and $x$}

For one observation $z_i \in \mathbb{R}$, $x_i \in \mathbb{R}^p$,
$y_i \in \mathbb{R}$ (and dropping $i$ subscript for simplicity),
assume
\begin{align}
  (z \mid x) &\sim \N(\gamma^\trans x, \sigma^2_\nu) \\
  x &\sim \N_p(\mu, \Omega)
\end{align}
so the joint distribution is
\begin{align*}
  \begin{bmatrix}
    z \\
    x
  \end{bmatrix} &\sim \N_{p+1} 
                  \left(
                  \begin{bmatrix}
                    \gamma^\trans \mu \\
                    \mu 
                  \end{bmatrix},
  \begin{bmatrix}
    \gamma^\trans \Omega \gamma + \sigma^2_\nu & \gamma^\trans \Omega \\
    \Omega^\trans \gamma & \Omega
  \end{bmatrix}
                  \right)
\end{align*}
Let $w = [z \quad x^\trans]^\trans$, and w.l.o.g., assume that
$\mu = 0$ so that $\E(w) = 0$.  Then denote the covariance of the
joint distribution with
\begin{align*}
  \Lambda &:= \text{cov}(w) = \begin{bmatrix}
    \gamma^\trans \Omega \gamma + \sigma^2_\nu & \gamma^\trans \Omega \\
    \Omega^\trans \gamma & \Omega
  \end{bmatrix}
\end{align*}

We will project estimates of the treatment effect $\alpha$ onto the
reduced $q$-vector of covariates $\wt$ after removing the last
$(p + 1 - q)$ covariates $\wdee$, i.e.
$w^\trans = [\wt^\trans \quad \wdee^\trans]$.  Note that the first
element of both $w$ and $\wt$ is $w_1 = \wt_1 = z$.  Then let
$\Lambdat = \cov(\wt)$, $\Lambdad = \cov(\wdee)$, and
$\Lambdadt = \cov(\wt, \wdee)$, inducing the block partition
\begin{align*}
  \Lambda &=
            \begin{bmatrix}
              \Lambdat & \Lambdadt \\
              \Lambdadt^\trans & \Lambdad
            \end{bmatrix}.
\end{align*}

\paragraph{Joint of $w$ and $y$}

With $w = [z \quad x^\trans]^\trans$ and $\psi = [\alpha \quad \beta^\trans]^\trans$,
so then
\begin{align*}
  (y \mid w) &\sim \N(\psi^\trans w, \sigma^2_\epsilon) \\
  w &\sim \N_{p+1}(\phi, \Lambda)
\end{align*}
so the joint distribution is
\begin{align*}
  \begin{bmatrix}
    y \\
    w
  \end{bmatrix} &\sim \N_{p+2} 
                  \left(
                  \begin{bmatrix}
                    \psi \phi \\
                    \phi
                  \end{bmatrix},
  \begin{bmatrix}
    \psi^\trans \Lambda \psi + \sigma^2_\epsilon & \psi^\trans \Lambda \\
    \Lambda^\trans \psi & \Lambda
  \end{bmatrix}
                  \right)
\end{align*}

\paragraph{Projection}

After $n$ observations of $z$, $x$, and $y$, let $X$ be the
$n \times p$ matrix of $x$ values, $Z$ is the $n$-vector of $z$
values, $Y$ is the $n$-vector of $y$ values, and $p$.

Consider the matrix $\Xt$ of reduced columns of $X = [\Xt \quad \Xd]$
(i.e., remove the $\Xd$ columns of $X$) with corresponding vector
$\betat$, and corresponding concatenations $\Wt = [Z \quad \Xt]$ and
$\psit = [\alpha \quad \betat]$, and for simplicity let
$W_\dagger = X_\dagger$.  The projection is performed via
\begin{align*}
  \psit &= \underbrace{(\Wt^\trans \Wt)^{-1} \Wt^\trans W}_{A} \psi
\end{align*}
% and so the projected posterior has the form
% \begin{align*}
%   (\tilde \psi \mid Y) &\sim \N(P\hat{\psi}, \sigma_\epsilon^2 P
%                           (W^\trans W)^{-1} P^\trans).
% \end{align*}

Note that $A$ can be simplified to
\begin{align*}
  A &= (\Wt^\trans \Wt)^{-1} \Wt^\trans W \\
    &= (\Wt^\trans \Wt)^{-1} \Wt^\trans [\Wt \quad W_\dagger] \\
    &= [\I \quad (\Wt^\trans \Wt)^{-1} \Wt^\trans W_\dagger]
\end{align*}

%%% Local Variables:
%%% mode: latex
%%% TeX-master: "../main"
%%% End:
