# Supplementary material for: Bayesian inference for treatment effects under nested subsets of controls
Source: arXiv:2001.07256 source file (2022-09-02)
Supplement: Supplementary file 3 [file wang-monte-carlo.tex]

\section{Replications of Wang et al. simulation example}
\label{sec:replications-wang-et}

Figure~\ref{fig:wang-ONEDATASET} and \ref{fig:wang-ONECHAIN} show
Monte Carlo variance in the solution path coming from the data
generating mechanism and the posterior sampling scheme.

\begin{figure}[ht]
  \centering
  \includegraphics[width=0.8\textwidth]{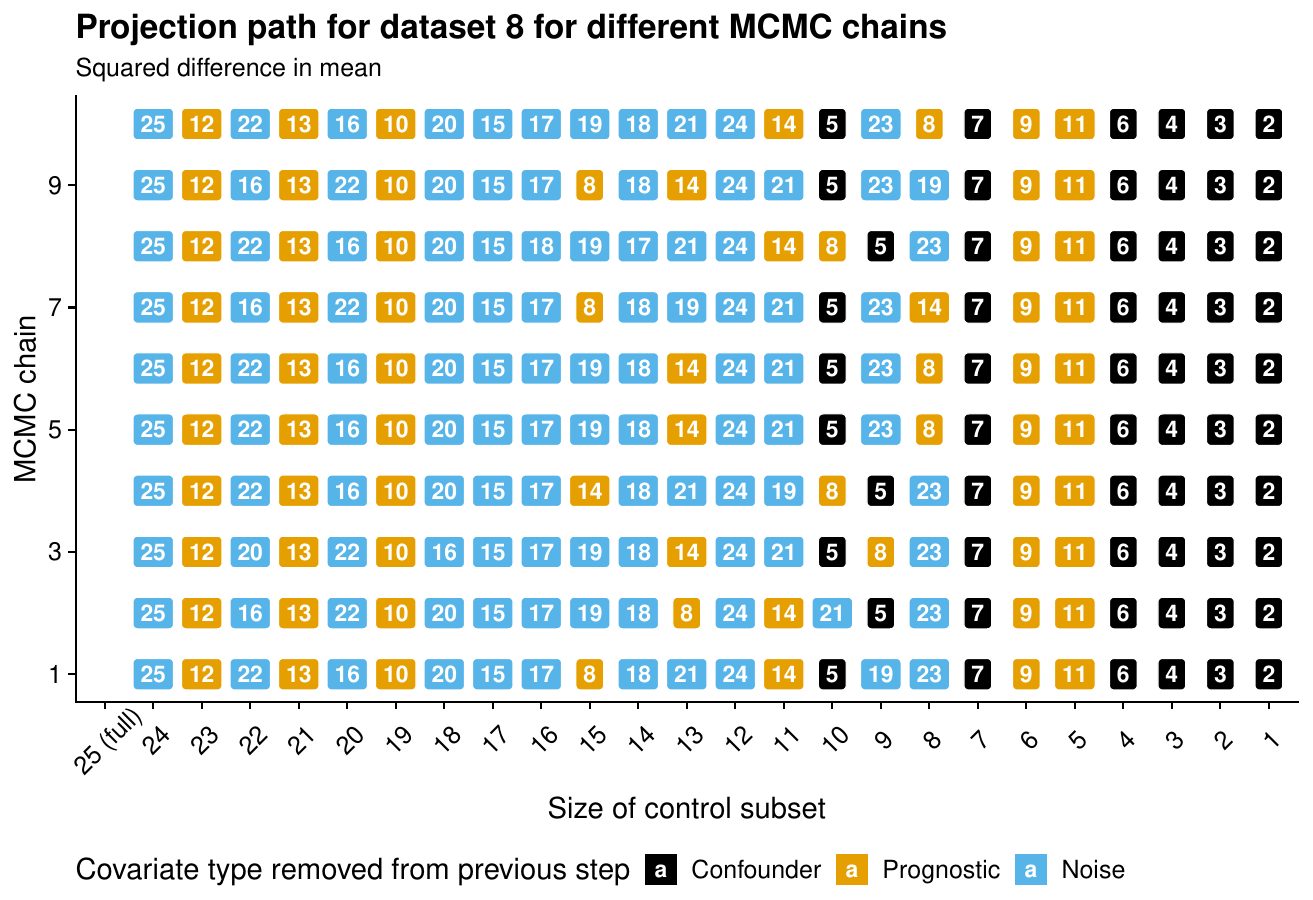}
  \caption{\label{fig:wang-ONEDATASET} Results of simulation example
    from Wang et al., showing summary path for ten independent sets of
    posterior samples from one dataset. }
\end{figure}

% \begin{figure}[ht]
%   \centering
%   \includegraphics[width=0.8\textwidth]{figures/wang-labelPlotONECHAIN.pdf}
%   \caption{\label{fig:wang-ONECHAIN} Results of simulation example
%     from Wang et al., showing summary path for one set of posterior
%     samples from each of 10 different datasets generated from the same
%     model. }
% \end{figure}

%%% Local Variables:
%%% mode: latex
%%% TeX-master: "../main"
%%% End:
